# Supplementary material for: PNeRV: Enhancing Spatial Consistency via Pyramidal Neural Representation for Videos
Source: arXiv:2404.08921 source file (2024-04-13)
Supplement: Supplementary file 4 [file supp_bak.tex]

\clearpage
\setcounter{page}{1}
\setcounter{section}{0}
\setcounter{table}{0}
\setcounter{figure}{0}
\setcounter{theorem}{0}
\setcounter{definition}{0}
\setcounter{lemma}{0}
\setcounter{proposition}{0}
\setcounter{remark}{0}
\setcounter{problem}{0}

\renewcommand\thesection{\Alph{section}}
\maketitlesupplementary
\renewcommand\thefigure{\thesection{}.\arabic{figure}}
\renewcommand\thetable{\thesection{}.\arabic{table}}
\renewcommand\thetheorem{\thesection{}.\arabic{theorem}}
\renewcommand\thedefinition{\thesection{}.\arabic{definition}}
\renewcommand\theproposition{\thesection{}.\arabic{proposition}}
\renewcommand\thelemma{\thesection{}.\arabic{lemma}}
\renewcommand\theremark{\thesection{}.\arabic{remark}}
\renewcommand\theproblem{\thesection{}.\arabic{problem}}

The appendix includes more discussions on theoretical analysis and related works, additional results and ablation studies.

\section{More Discussions of Universal Approximation Theory (UAT) Analysis on NeRV}
We provide more analysis and discussions of UAT analysis on NeRV system. We define the problem that current NeRV systems are attempting to address, and provide a comparison with existing video neural coding pipelines.

\subsection{Implicit Neural Video Coding Problem}\label{app_uat}
Following the pipeline of Implicit Neural Video Coding (INVC) which presented in Sec. 4.2%~\ref{invc_sec}
, we recall the proposed Implicit Neural Video Coding Problem (INVCP) as follow.
\begin{problem}(INVC Problem).\label{IVNCP}
The goal for Implicit Neural Video Coding is to find out the optimal design of decoder $\mathcal{D}$ and encoder $\mathcal{E}$ in pursuit of minimal parameter quantity $\mathsf{Param}(\mathcal{D})$ and embeddings $ \{ e_{t}=\mathcal{E} \left( t \right) \in \mathbb{R}^{d_{in}^t} \}^{T}_{t=1}$ (where $d = d^{t}_{in}$ is often equal among $t$ in existing NeRV systems) under certain approximation error $\epsilon$ between reconstruction $\tilde{V}$ and given video sequence $V$,
\begin{gather}\label{IVNC}
\mathop{\arg\min}_{\mathcal{D}, \mathcal{E} }~ \mathsf{Param} \left( \mathcal{D} \right) + \sum_{t=1}^{T} d_{in}^t , \nonumber  \\
\mathrm{ s.t. } ~ L_{\mathcal{D}}, w_{\mathcal{D}} \in \left[1, \infty \right),~\mathop{\sup} \mathop{\sum} \Vert \tilde{V_t} - V_t\Vert \leq \epsilon,~t \in [1, T]. \notag
\end{gather}
\end{problem}
In the practise of INVC research, we usually use the dual problem of~\ref{IVNCP} to find out the optimal architecture of a model to fit the video under certain error, named as Dual Implicit Neural Video Coding Problem (DINVCP).
\begin{problem}(Dual INVC Problem).\label{DIVNCP}
Given the certain parameter quantity $\mu$, Dual INVC problem tries to find out the optimal design of decoder $\mathcal{D}$ and encoder $\mathcal{E}$ to approach the minimal approximation error between reconstruction $\tilde{V}$ and given video sequence $V$,
\begin{gather} \label{DIVNC}
%\mathop{\arg\min}_{\mathcal{D}, \mathcal{H} }~\mathop{\sup} \Vert \mathcal{G}(t) - \mathcal{V}(t) \Vert, \nonumber  \\
\mathop{\arg\min}_{\mathcal{D}, \mathcal{E} }~\mathop{\sup} \mathop{\sum} \Vert \tilde{V_t} - V_t\Vert, \nonumber  \\
\mathrm{ s.t. } ~ L_{\mathcal{D}}, w_{\mathcal{D}} \in \left[1, \infty \right), \mathsf{Param} \left( \mathcal{D} \right) + \sum_{t=1}^{T} d_{in}^t \leq \mu ,~t \in [1, T].\notag
\end{gather}
\end{problem}

In practise, when using a NeRV model to represent a given video under certain model size limit $\mu$ through end-to-end training, it is trying to solve the DINVCP.


\subsection{Comparison between DINVCP and Previous Neural Coding Pipelines}
Distribution-Preserving Lossy Compression (DPLC) is proposed by~\cite{Tschannen2018DeepGM} motivated by GAN-based image compression~\cite{Agustsson2018GenerativeAN}, and is given as
\[
%\min_{E,D}~~ \mathbb{E}_{X,D} [d(X,D(E(X)))],~s.t.~~D(E(X))\sim X,
\min_{E,D}~~ \mathbb{E}_{X,D} [d(X,D(E(X)))] + \lambda d_f(p_X,p_{\tilde{X}}),
\]
where $E, D, X, \tilde{X}$ are encoder, decoder, given input and reconstruction, $d_f$ is a divergence which can be estimated from samples. DPLC believes that it is important to keep distribution consistent for compression and reconstruction. 


\cite{rdo} proposes the Rate-Distortion Optimization (RDO). Later, \cite{Blau2017ThePT} reveals the importance of perceptual quality and propose the Perception-Distortion Optimization (PDO) as
\[
\min_{p_{\tilde{X}|Y}}~ d(p_X, p_{\tilde{X}})~~s.t.~~ \mathbb{E}[\Delta(X, \tilde{X})] \leq D,
\]
where $\Delta$ is distortion measure and $d$ is divergence between distributions. Further, \cite{Blau2019RethinkingLC} defines the Rate-Distortion-Perception Optimization (RDPO) as
\[
%R(D,P)=\min_{p_{\tilde{X}|X}} I(X, \tilde{X})~~s.t.~~ \mathbb{E}[\Delta(X, \tilde{X})] \leq D,~d(p_X, p_{\tilde{X}}) \leq P,
\min_{p_{\tilde{X}|X}} I(X, \tilde{X})~~s.t.~~ \mathbb{E}[\Delta(X, \tilde{X})] \leq D,~d(p_X, p_{\tilde{X}}) \leq P,
\]
where $I$ denotes mutual information. 


\iffalse
Recall that Dual INVC problem (DINVCP) is
\begin{gather} \label{DIVNC}
\mathop{\arg\min}_{\mathcal{D}, \mathcal{H} }~\mathop{\sup} \Vert \mathcal{G}(t) - \mathcal{V}(t) \Vert, \nonumber  \\
\mathrm{ s.t. } ~ L_{\mathcal{D}}, w_{\mathcal{D}} \in \left[1, \infty \right), \mathsf{Param} \left( \mathcal{D} \right) + \sum_{t=1}^{T} d_{in}^t \leq p ,~t \in [1, T],
\end{gather}
where $\mathcal{V}$ is given video, $\mathcal{G}=\mathcal{D} \circ \mathcal{H}$ is NeRV system consisting of encoder $\mathcal{H}$ and decoder $\mathcal{D}$ which has finite length $L_{\mathcal{D}}$ and width $w_{\mathcal{D}}$. The embedding in $t$-th time stamp is generated by $\mathcal{H}$ in the shape of $d_{in}^t \times 1$.
\fi

The primary objective, which also serves as the main obstacle in the aforementioned pipelines, is that density estimation is not only costly but also challenging to estimate accurately.
Different from DPLC, RDO, PDO or RDPO, \textit{DINVCP does not need to model the distribution of the given signal explicitly.} In fact, the distribution of input images or videos is difficult to approximate, whether it is approached by minimizing ELBO or adversarial training~\cite{vae, gan}, there is always a certain gap or mismatch. Besides, other density estimation methods such as flow-based models or diffusion models suffer from huge computational costs~\cite{ddpm, ldm}. In contrast, \textit{NeRV system implicitly models the unknown distribution of given signal via specific decoding computation process under certain model parameter quantity. The calculation process per se is regarded as the side information}~\cite{Wyner1976TheRF, Jonschkowski2015PatternsFL}. 

This approach of implicitly modeling distributions through computational processes under parameter quantity constraints aligns with some current perspectives that suggest the intelligence of Large Language Models (LLM) stems from the data compression~\cite{cagi, Deletang2023LanguageMI}. LLMs such as GPT aim to transfer as much data as possible to models of the same size for learning (and continue to increase the model size after learning), in order to achieve information compression and efficient information coding. However, NeRV system strives to compress the model size as much as possible at similar data levels, achieving efficient representation of data

The improvement of PNeRV on perceptual quality actually confirms this conjecture. By upgrading the model structure, PNeRV realizes better perceptual performance without estimating the unobtainable prior distribution of signal.





%\subsection{Proof of Theorem~\ref{param}}\label{app_a}
\subsection{Proof of Theorem 1}\label{app_a}
Following the definitions given in Sec. 4%~\ref{uat_sec}
, the width $w$ of $\mathcal{N}$ is named as $\mathop{\max} d_i, \{ d_i \in \mathbb{N} \}^L_{i=1}$. Once the minimal width $w^* = w_{min} \left( d_{in}, d_{out}\right)$ is estimated by $d_{in}, d_{out}$, such that, for any continuous function $f: [0,1]^{d_{in}} \to \mathbb{R}^{d_{out}}$ with $\epsilon \geq 0$, there exists a $\mathcal{N}$ with input dimension $d_{in}$, hidden layer widths at most $w^*$, and output dimension $d_{out}$ that $\epsilon-$approximates $f$:
\[
\mathop{\sup}_{x \in [0,1]^ {d_{in}}} \Vert f \left(x \right) - \mathcal{N} \left(x \right) \Vert \leq \epsilon.
\]
The goal of Theorem 1%~\ref{param}
is to determine the minimum parameter demand when $\epsilon-$approximates the implicit $\mathcal{F}$ which represents the given video. We recall Theorem 1%~\ref{param}
as Theorem~\ref{param_app} as follow for better illustration.

\begin{theorem}\label{param_app}
For a cascaded NeRV system to $\epsilon$-approximate a video $V$ which is implicitly characterized by a certain unknown L-lipschitz continuous function $\mathcal{F}: K \to \mathbb{R}^{d_{out}}$ where $K \subseteq \mathbb{R}^{d_{in}}$ is a compact set, then the upper bound of the minimal parameter quantity $\mathsf{Param}(\mathcal{D})$ is given as\vspace{-0.02in}
\[
 \mathsf{Param}_{\min}(\mathcal{D})\leq d_{out}^2 \left( \frac{ \mathop{O}
    \left(diam  \left(K \right)
    \right) }{\omega_\mathcal{F}^{-1} \left( \epsilon \right) }
\right)^{d_{in}+1}.
\]
\end{theorem}


Before we start, we will recall the setup and demonstrate some mathematic concepts and lemmas.
\begin{definition}\label{string}
A function $g : \mathbb{R}^{d_{in}} \to \mathbb{R}^{d_{out}}$ is a max-min string of length $L \geq 1$ on $d_{in}$ input variables and $d_{out}$ output variables if there exist affine functions ${\ell}_1, \cdots ,{\ell}_L: \mathbb{R}^{d_{in}} \to \mathbb{R}^{d_{out}}$ such that
\[
g = \sigma_{L-1} ( \ell_L, \sigma_{L-2} \left(  \ell_{L-1},\cdots , \sigma_2 \left( \ell_3, \sigma_1\left( \ell_1, \ell_2\right)\right) \cdots \right).
\]
\end{definition}


The definition of max-min string and DMoC (Def. 3%~\ref{moc}
) are first introduced in~\cite{UniversalFA} and~\cite{ApproximatingCF}. We introduce two lemmas which given as Propositions 2 and 3 in~\cite{ApproximatingCF}.
\begin{lemma}\label{L1}
For every max-min string $g$ on $d_{in}$ input variables and $d_{out}$ output variables with length $L$ and every compact $K \subseteq \mathbb{R}^{d_{in}}$, there exists a \textsc{ReLU} net $\mathcal{N}$ with input dimension $d_{in}$, hidden layer width $d_{in}+d_{out}$, and depth $L$ that computes $x \mapsto g(x)$ for every $x \in K$.
\end{lemma}

\begin{lemma}\label{L2}
For every compact $K \subseteq \mathbb{R}^{d_{in}}$, any continuous $f : K \to \mathbb{R}^{d_{out}}$ and each $\epsilon \geq 0$ there exists a max-min string $g$ on $d_{in}$ input variables and $d_{out}$ output variables with length
\[
\left( \frac{ \mathop{O}
    \left(diam  \left(K \right)
    \right) }{\omega_f^{-1} \left( \epsilon \right) }
\right)^{d_{in}+1},
\]
for which
\[
\Vert f-g \Vert_{C^0(K)} \leq \epsilon.
\]
\end{lemma}
%Differ from the minimal width which is desired to approach in universal approximation research, we pay more attention to these two lemmas when applying to NeRV system. Lemma~\ref{L1} is essentially the Lemma 4 in~\cite{UniversalFA} and Lemma~\ref{L2} is proposed in~\cite{ApproximatingCF} as Proposition 3. The proof details could be found in corresponding paper.



\begin{proof}
From Lemma~\ref{L2}, the implicit function $\mathcal{F}_{\mathcal{V}}$ which represents the video $\mathcal{V}$ can be approximated by one max-min string $g$ which defined in~\ref{string}. It is worth mentioning that $\mathcal{F}_{\mathcal{V}}$ is supposed to be continuous because video can be considered as a slice of Minkowski space in real life. The length of the max-min string $g$ is given by Lemma~\ref{L2}. According to Lemma~\ref{L2}, there exists a \textsc{ReLU} net $\mathcal{N}_g$ with same input and output dimensions that fit the max-min string. So, the minimal parameters of $\mathcal{N}_g$, also the sum of weights for each affine layer, is
\[
\mathbf{Param} =\sum_{l=1}^{L} w_l w_{l-1},
\]
where $L$ is given in Lemma~\ref{L2}. Further the minimal width $w_{\min}$ is estimated as $\max\{d_{in}+1, d_{out} \}$ by~\cite{MinimumWF} (Lemma~1%\ref{L3}
), thus the minimal parameters of $\mathcal{N}_g$ under certain error is no longer than
\begin{equation}
\begin{split}
\mathbf{Param}_{\min} & \leq w_{\min}^2 \left( \frac{ \mathop{O}
    \left(diam  \left(K \right)
    \right) }{\omega_f^{-1} \left( \epsilon \right) }
\right)^{d_{in}+1} \nonumber \\
& = d_{out}^2 \left( \frac{ \mathop{O}
    \left(diam  \left(K \right)
    \right) }{\omega_f^{-1} \left( \epsilon \right) }
\right)^{d_{in}+1}, \nonumber
\end{split}
\end{equation}
where $w_{\min}= d_{out}$ for video $\mathcal{V}: \mathbb{N}\to \mathbb{R}^{d_{out}}$. Equality is reached when each layer width reaches the upper bound of minimal width.
\end{proof}

\begin{remark}\label{r1}
Although the upper bound of $\mathsf{Param}(\mathcal{D})$ is fixed regardless of detailed architecture, the actual performance of serial NeRV will be influenced by structure design, parameter initialization, activation functions, loss functions and optimizer. %We will only use Theorem~\ref{param} as a guide to improve NeRV.
\end{remark}




\section{More Related Works}
%Due to the extensive research scope of the theory or neural network architecture involved in this article, we will discuss more other research related to this paper. We add additional references, which may result in the references number being different from the main body.

\noindent\textbf{Comparison with other Subpixel-based Upsampling Operators}. NeRV system aims at reconstructing high-resolution videos through decoding the low-dim embeddings, thus proper upsampling operators are crucial for the performance. Existing subpixel-based upsampling operators are not efficient enough for NeRV system. Deconv~\cite{deconv} pads the subpixels by 0 and then pass through the Conv layer, resulting in block artifacts~\cite{deconv_arti}. PixelShuffle~\cite{ps} first expands the feature map channels through \textsc{Conv}, and then rearranges them into target subpixels. However, the desired subpixels of one position is only related to the expanding channels of the same position, ignoring context information, shown in Fig.~2%\ref{ps_kfc}
~of the main text. Also, PixelShuffle will encounter an exponential explosion of required channels when the upsampling ratio is large. 


\noindent\textbf{Comparison with INR on Image}.~\cite{siren} (SIREN) uses sine as a periodic activation function to model the high-frequency information of a given image~\cite{fourier} and conducts a sinusoidal transformation prior to input. \cite{Xu_2022_INSP} tries to directly modify an INR without explicit decoding. The main difference between these methods and ours is that we consider the input coordinate-pixel pairs to be \textit{dense} for the INR on image coding. In a natural image, the RGB value at a specific position is often closely related to its neighboring positions. However, for high-resolution video, the gap between adjacent frames can be much larger, both in pixel and semantic terms. This situation is more akin to only observing partial pixels from a given image. 

%We have not yet addressed the issue of high-frequency detail recovery in videos, but we intend to explore this area further in future research.


%\noindent\textbf{Comparison with other Kronecker Factorization-based Models}. \cite{Tahaei2021KroneckerBERTLK} proposes a model compression method using Kronecker decomposition and adopt it in all linear mappings in the Transformer layer~\cite{AttentionIA}. Also, \cite{Jose2017KroneckerRU} decomposes the weight metrices $W$ in RNN into $W = \otimes_{f=0}^{F-1} W_f$. The main difference between them and our method is that \textsc{KFc} also needs to compute the bias term in an efficient manner. We add the lightweight bias calculation via CP decomposition and first adopt the Kronecker decomposition-based operation to the NeRV research.

\iffalse
\noindent\textbf{Comparison with Bilinear Feature Fusion}. The calculation of \textsc{KFc} seems similar to the multi-head graph attentional layer (GATs)~\cite{gatn}, but they are different. The final output of graph attention between $N$ node features $h_j$ and normalized attention coefficients $\alpha$ is calculated as
\[
h_i^{'} = \sigma \left( \sum_{j \in N} \alpha_{ij} \mathbf{W} h_j \right),
\]
where $W$ is the weight metrix. It calculates the global correlation between features in each node. GATs and \textsc{KFc} both have a global receptive field to given features, but another main goal of \textsc{KFc} is to upscale the shape efficiently. The mechanism of \textsc{KFc} is the kronecker decomposition of fully-connected layer and \textsc{KFc} is only formally like GATs or other bilinear models~\cite{Li2016FactorizedBM}. The principal aim of bilinear models is to calculate the relationship between two diverse vectors.
\fi


\noindent\textbf{Comparison with Self-attention Module}. Self-attention (SA) and Multi-head Self-attention (MSA) module~\cite{NonlocalNN, AttentionIA, SwinTH, t2023is} computes the response at a position by attending to all positions, which is similar to \textsc{KFc}. The major defect of SA and MSA when adopted in NeRV is that the computational complexity and the space complexity are too high to efficiently compute the global correlations between arbitrary positions, especially the computational cost ($O(n^2 d)$) between queries and keys for high resolution feature maps. \textsc{KFc} not only captures long-range dependencies but also achieves low-cost rescaling, both of which are significant to NeRV.





\section{Additional Results}
All models utilized in the additional results are trained by a 3M model in 300 epochs unless otherwise clarified.
\subsection{Comparison of Generalization Ability by Video Interpolation Results}\label{app_int}
Indeed, the concepts of approximation and generalization are distinct topics within the field of deep learning theory~\cite{Nakkiran2019DeepDD, Advani2017HighdimensionalDO}. Understanding the causal relationship between overfitting and the generalization capacity of NeRV necessitates further investigation. Existing NeRV models always concentrate on the models' approximation capabilities through overfitting training. 

Nonetheless, we also evaluate the generalization performance of our proposed PNeRV through video interpolation experiment. Adhering to the experimental methodology employed in the \cite{HNeRV} and \cite{DNeRV}, the model is trained using odd-numbered frames and then tested with unseen even-numbered frames. The results, presented in Table~\ref{int}, indicate that PNeRV surpasses most of the baseline methods. Future research will focus on the theoretical analysis and enhancement of PNeRV's generalization abilities.


\begin{table*}[h]
    \setlength{\tabcolsep}{3pt}
  \centering\small
      \setlength{\abovecaptionskip}{0.05in}
      \setlength{\belowcaptionskip}{-0.05in}
  \begin{tabular}{l|lllllll|c}
 %\toprule
     PSNR         & Beauty & Bospho & Honey & Jockey & Ready & Shake &Yacht &Avg.\\
    \midrule[1.5pt]
    NeRV~\cite{nerv}     &28.05  & 30.04 & 36.99  &20.00 &17.02  & 29.15  &24.50 & 26.54 \\
    E-NeRV~\cite{enerv}  &27.35  & 28.95 & 38.24  &19.39 &16.74  & 30.23  &22.45 & 26.19 \\
    H-NeRV~\cite{HNeRV}  &31.10  & 34.38 & 38.83  &23.82 &20.99  & 32.61  &27.24 & 29.85 \\
    DiffNeRV~\cite{DNeRV}&35.99  & 35.10 & 37.43  &30.61 &24.05  & 35.34  &28.70 & \textbf{32.47} \\
 \midrule
    PNeRV                &33.64  & 34.09 & 39.85  &28.74 &23.12  & 31.49  &27.35 & \underline{31.18} \\
  % \bottomrule[1.5pt]
  \end{tabular}
    \caption{Video interpolation results on 960 $\times$ 1920 UVG in PSNR.}
  \label{int}
\end{table*}

\iffalse
\subsection{Perceptual Comparison}
We report the LPIPS~\cite{LPIPS} distance of PNeRV (PNeRV-M in 3M and PNeRV-L in 3.3M) comparied with the previous SOTA method (DiffNeRV~\cite{DNeRV} in 3.3M) in Tab.~\ref{LPIPS}. LPIPS is given by a weighted L2 distance between deep features of frames and the AlexNet~\cite{alexnet} which pretrained on ImageNet is used as the deep feature extractor.

Under the same conditions, although the average PSNR of DiffNeRV is only 1.14\% worse, but the average LPIPS is 4.83\% worse than the PNeRV-L. The results indicate that the reconstruction of proposed methods is better under the perspective of human visual perception. With the help of high-level information interaction, the proposed PNeRV is more likely to be beneficial for downstream video classification, semantic segmentation, object detection or other semantic-level visual tasks. We would discuss it further in Fig.~\ref{bsm_1} and~\ref{bsm_2}.


\begin{table}[h]\scriptsize
    \tabcolsep=0.08cm
      \setlength{\abovecaptionskip}{5pt}
      \caption{LPIPS comparison on UVG. LPIPS is calculated by trained model which its PSNR is on the right. Avg. is the average LPIPS on whole UVG, the lower the better.}
      \resizebox{!}{0.83cm}{\centering
  \begin{tabular}{l|lllllll|c}
 %\toprule
     LPIPS/PSNR         & Beauty & Bospho & Honey & Jockey & Ready & Shake &Yacht &Avg.\\
    \midrule[1.5pt]
    DiffNeRV~\cite{DNeRV}  &0.205/40.00 &0.164/36.58 &0.042/41.97 &0.164/35.75 &0.206/28.16 &0.181/36.53 &0.241/30.43 &0.172/35.63\\
    PNeRV-M                &0.201/39.08 &0.160/35.56 &0.038/42.59 &0.271/31.51 &0.325/25.94 &0.154/37.61 &0.238/30.27 &0.198/34.65\\
    PNeRV-L                &0.210/38.94	&0.132/36.68 &0.037/42.73 &0.177/35.81 &0.211/28.97 &0.146/38.25 &0.230/30.92 &\textbf{0.163}/36.04\\
  % \bottomrule[1.5pt]
  \end{tabular}}
  \label{LPIPS}
\end{table}


\begin{figure}[h]
    \centering
	\begin{minipage}{0.45\linewidth}
   \setlength{\belowcaptionskip}{-0.05in}
  \resizebox{!}{0.7\linewidth}{\centering
  \includegraphics[width=1\linewidth]{UVG_msssim6.png}}\\
  %\vspace{-0.05in}%\caption{a}
  %\label{ssim}%\vspace{-0.05in}
	\end{minipage}
	\begin{minipage}{0.45\linewidth}
  %\raisebox{-0.15\height}{
  \resizebox{!}{0.7\linewidth}{\centering
  \includegraphics[width=1\linewidth]{train.png}}
  %}
  \\ %\caption{b}
   % \label{train}%\vspace{-0.05in}
	\end{minipage}
\vspace{-0.05in}\caption{Left: Comparison of video compression on UVG in MS-SSIM. Right: Example of training failure of different NeRV methods in 3M size.}\label{train}
\end{figure}
\fi




\begin{figure}[t]
  \centering
  %\subfigure{
  	\begin{minipage}{1\linewidth}
     \setlength{\belowcaptionskip}{-0.05in}
		\centering
  \includegraphics[width=0.8\linewidth]{comp.png}%\\
  %\vspace{-0.05in}
  \caption{PSNR of video compression on UVG.}
  \label{comp_p}%\vspace{-0.05in}
   \end{minipage}
   %}
   \hfill
  %\subfigure{
  \begin{minipage}{1\linewidth}
  \centering
  \includegraphics[width=0.8\linewidth]{UVG_msssim6.png}%\\
  %\vspace{-0.05in}
  \caption{SSIM of video compression on UVG.}
  \label{comp_s}%\vspace{-0.05in}
   \end{minipage}
   %}
\end{figure}


\begin{figure}[h]
    \centering
         \setlength{\belowcaptionskip}{-0.05in}
	%\begin{minipage}{0.45\linewidth}
  %\resizebox{!}{0.7\linewidth}{
  %\centering
  %\includegraphics[width=1\linewidth]{UVG_msssim6.png}
  %}
  %\\
  %\vspace{-0.05in}%\caption{a}
  %\label{ssim}%\vspace{-0.05in}
	%\end{minipage}
	%\begin{minipage}{0.45\linewidth}
  %\raisebox{-0.15\height}{
  %\resizebox{!}{0.7\linewidth}{\centering
  \includegraphics[width=0.8\linewidth]{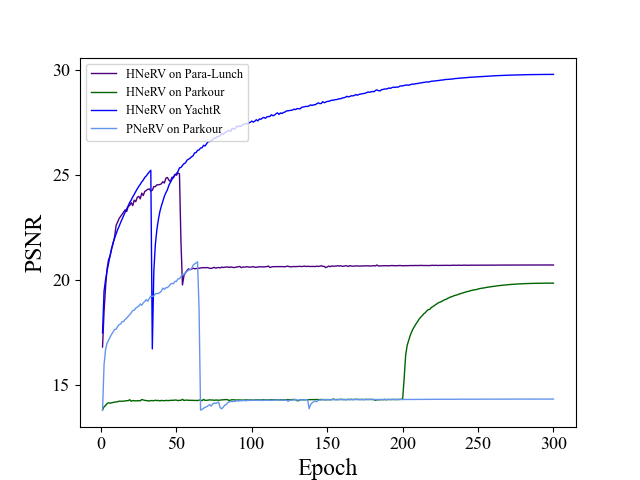}
  %}
  %}
  %\\ %\caption{b}
   % \label{train}%\vspace{-0.05in}
	%\end{minipage}
\vspace{-0.05in}\caption{%Left: Comparison of video compression on UVG in MS-SSIM. Right: 
Example of training difficulty of different NeRV methods in 3M size.}\label{train}
\end{figure}




\begin{table*}[!t]
	\noindent
     \setlength{\abovecaptionskip}{0.05in}
     \setlength{\belowcaptionskip}{-0.05in}
	\begin{minipage}{0.3\textwidth}
		\centering
  \resizebox{!}{0.6cm}{
		\begin{tabular}{c||ccc}
                & 40$\times$80  & 20$\times$40 & 10$\times$20 \\
        \midrule[1.2pt]
        PSNR    &\textbf{31.94} & 31.33 &30.50\\
        MS-SSIM &\textbf{0.960} & 0.954 &0.947\\
       %\midrule[1.5]
        \end{tabular}
        }
		\caption{Embedding size in PNeRV-L.}
		\label{abla_1}
         \end{minipage}
	\begin{minipage}{0.3\textwidth}
		\centering
	  \resizebox{!}{0.6cm}{
		\begin{tabular}{c||ccc}
         & 1$\times$1 & 3$\times$3  & 5$\times$5  \\
        \midrule[1.2pt]
        PSNR    &31.92 & \textbf{31.94}& 31.90\\
        MS-SSIM &0.960 &0.960 & \textbf{0.961} \\
       %\midrule[1.5]
         \end{tabular}
         }
       	\caption{Kernel size in BSM.}
		\label{abla_2}
	\end{minipage}
 	\begin{minipage}{0.3\textwidth}
		\centering
  \resizebox{!}{0.6cm}{
 \begin{tabular}{c||ccc|c}
               & ReLU & Leaky & GeLU & w/o BN\\
        \midrule[1.2pt]
        PSNR &    31.80 & 31.86 & \textbf{31.94} &31.53\\
        MS-SSIM &0.959& \textbf{0.961} &0.960 & 0.959\\
        %\bottomrule[1.2pt]
         \end{tabular}
         }
		\caption{Activation and BN in \textsc{KFc}.}
		\label{abla_3}
         \end{minipage}
\end{table*}





\subsection{Comparison of Video Compression and Discussion of Training Difficulty}\label{app_comp}
The video compression comparison of PNeRV with other NeRV models in PSNR and MS-SSIM is shown in Fig.~\ref{comp_p} and Fig.~\ref{comp_s}. Following the same setting utilized in~\cite{HNeRV, DNeRV}, we evaluate the video compression comparison with 8 bits quantization for both embeddings and model, without model pruning. 

PNeRV outperforms traditional pipelines~\cite{h264, h265}, other implicit methods~\cite{nerv, enerv, HNeRV, DNeRV, divnerv} and several neural video coding models~\cite{dvc, MLVC, dcvc}. On the guidance of Remark~2%\ref{AtoP}
, we encode videos by models in adaptive size and named as \textit{Unified Compression Strategy} (UCS). For example, in 0.0384 Bpp we use models in 1.5M on videos with few motion but 3.3M for others. In other words, UCS applies different $d^t_{in}$ for $t$ in Problem.~\ref{DIVNCP}. The decoding FPS of PNeRV for $960 \times 1920$ video is 11.90, slower than DiffNeRV~\cite{DNeRV} (FPS 25.6) but much faster than DCVC~\cite{dcvc} (FPS 0.028).




It should be noted that, all implicit models suffer from the dramatic training difficulty under large parameters such as 5M or greater. Models will fall into local minima result in trivial outputs. This phenomenon seriously hinders the compression performance of all NeRV methods when Bpp gets larger. Some examples of failure training process are shown on the right of Fig.~\ref{train}, where models are 3M under the same conditions.




\subsection{More Visualization Examples for Perceptual Quality}\label{app_qual}
We show some more examples of qualitative comparisons between different models.

Shown in~\ref{add_davis}, the results of PNeRV are more smooth and less noisy. Such as ``Lucia'' and ``Horse-low'', PNeRV pays more attention to the geometric pattern of main objects and ignores those high-frequency details of the background scene. Other baseline methods could not reconstruct frames in such semantic level. Due to the lack of high-level information guidance and global receptive field, baseline methods are hard to reasonably allocate model weights to more important objects, e.g., red waterpipe in ``Breakdance-flare'' and patterns in ``Cows''.

Shown in~\ref{same_davis}, the comparison in different time stamp of same video indicates some specific common issues of different models.
Overlapping and noisy patterns are occurred in the results of DiffNeRV~\cite{DNeRV} and HNeRV~\cite{HNeRV} such as grass and hands in ``Hike''. ENeRV~\cite{enerv} and NeRV~\cite{nerv} often result in color deviation and blurring, e.g. backpack in ``Hike'' and motor in ``motor-bump''. PNeRV achieves a balance between preserving details and maintaining the semantic consistency. Compared to DiffNeRV, which also uses difference of frames as input, the latter's reconstruction of details is unbiased. However, in fact, human attention to visual elements under different semantics should be different. Improving the reconstruction results through high-level information is one of PNeRV's pursuits.

\subsection{Discussion on the Failure Cases}
As shown in Table~2%\ref{davis}
, PNeRV fails in ``Dog'' which is a blurred video mixed with jitter and deformation. Also, the ``Soapbox'' video, which contains two video clips from entirely different scenes connected by a few frames in which the camera rotates in a large angle. So far, PNeRV is not able to handle severe temporal inconsistency effectively.




\begin{table*}[!t]\footnotesize
      \centering
      %\belowrulesep=0pt
      %\aboverulesep=5pt
      \setlength{\abovecaptionskip}{0.05in}
      \setlength{\belowcaptionskip}{-0.05in}
       \tabcolsep=0.09cm
  %\resizebox{!}{1.2cm}{
  \centering
  \begin{tabular}{l||lllllll|c|c}
 %\toprule
     Models                   &Bmx-B & Camel & Dance-J & Dog & Drift-C & Parkour &Soapbox	 &Avg. &A.P.G \\
    \midrule[1.2pt]
    NeRV~\cite{nerv}  &29.42/0.864  &24.81/0.781  &27.33/0.794  &28.17/0.795 &36.12/0.969 &25.15/0.794 &27.68/0.848 &28.38/0.835 &-\\
    E-NeRV~\cite{enerv} &28.90/0.851  & 25.85/0.844 & 29.52/0.855 &30.40/0.882 &39.26/0.983  &25.31/0.845 &28.98/0.867 &29.75/0.875 &-\\
    HNeRV~\cite{HNeRV}  &29.98/0.872 & 25.94/0.851 &29.60/0.850 &30.96/0.898 &39.27/0.985  &26.56/0.851  &29.81/0.881 & 30.30/0.874 &-\\
    DiffNeRV~\cite{DNeRV} &30.58/0.890  & 27.38/0.887 &29.09/0.837 &\textbf{31.32/0.905} &40.21/0.987 & 25.75/0.827 &\textbf{31.47/0.912} &30.84/0.892 &-\\
 %\midrule
 \midrule[1.2pt]
    %\textit{Ablation Study on different upscaling operators and feature fusion modules. }\\
    \textit{Ablation Study} \\
 \midrule[1.2pt]
    Bilinear + Concat &24.85/0.783 &24.49/0.793 &28.32/0.806 &26.19/0.723 &31.92/0.943 &25.09/0.793 &29.23/0.872 &27.16/0.816 &\textcolor{red}{-4.07}\\
    Bilinear + GRU &29.86/0.874 &25.00/0.811 &29.16/0.830 &27.11/0.753 &32.09/0.945 &26.43/0.845 &29.10/0.874 &28.39/0.847 &\textcolor{red}{-2.84}\\
   Bilinear + LSTM &26.22/0.792 &26.87/0.871 &27.85/0.788 &26.71/0.741 &33.65/0.946 &25.82/0.820 &29.42/0.881 &28.07/0.834 &\textcolor{red}{-3.16}\\
    Bilinear + \textbf{BSM} &29.97/0.877 &27.35/0.881 &29.49/0.838 &27.14/0.756 &34.34/0.968 &26.15/0.835 &29.14/0.876 &29.08/0.862  &\textcolor{red}{-2.15}\\
 \midrule[0.1pt]
    DeConv + Concat &28.06/0.840 &24.07/0.774 &27.86/0.792 &25.16/0.693 &34.97/0.961 &22.13/0.683 &29.33/0.877 &27.37/0.803  &\textcolor{red}{-3.86}\\
    DeConv + GRU &27.52/0.827 &28.16/0.900 &29.09/0.825 &25.76/0.706 &37.91/0.980 &25.09/0.793 &29.54/0.882 &29.00/0.845  &\textcolor{red}{-2.23}  \\
   DeConv + LSTM &30.15/0.882 &26.49/0.859 &28.30/0.805 &25.94/0.712 &34.91/0.956 &26.35/0.842 &30.26/0.895 &28.91/0.850 &\textcolor{red}{-2.32}\\
   DeConv + \textbf{BSM} &31.56/0.906 &27.18/0.878 &29.77/0.847 &30.09/0.868 &36.03/0.971 &26.09/0.831 &29.00/0.872 &29.96/0.881 &\textcolor{red}{-1.27}\\
  \midrule[0.1pt]
  \textbf{KFc} + Concat &27.51/0.826 &25.02/0.816 &29.02/0.831 &28.80/0.831 &36.82/0.974 &25.12/0.796 &28.53/0.864 &28.68/0.848 &\textcolor{red}{-2.55}\\
  \textbf{KFc} + GRU &\textbf{31.69/0.910} &25.88/0.848 &28.32/0.805 &28.47/0.813 &33.25/0.942 &26.68/0.853 &30.89/0.903 &29.31/0.868 &\textcolor{red}{-1.92}\\
 \textbf{KFc} + LSTM &29.16/0.862 &27.24/0.878 &28.90/0.825 &29.28/0.842 &32.73/0.935 &26.62/0.839 &29.35/0.879 &29.04/0.866 &\textcolor{red}{-2.19}\\ %\rowcolor{gray!40}
 \textbf{KFc} + \textbf{BSM} (\textbf{PNeRV})   &31.05/0.896  & \textbf{27.89/0.892} & \textbf{30.45/0.873} &31.08/0.898 &\textbf{40.23/0.987}  &\textbf{27.08/0.867} &30.85/0.902 & \textbf{31.22/0.902} & \textcolor{blue}{+0}\\
  %\bottomrule[1.2pt]
  \end{tabular} %}
  %\setlength{\belowcaptionskip}{-5pt}
%\vspace{-0.05in}
   \caption{Ablation results on DAVIS subset in PSNR and MS-SSIM, where Avg. is the average PSNR and A.P.G is the average PSNR gap. Every result is reported by corresponding model trained in 300 epoch and 3M size.
 }  \label{davis_abla_detail}
\end{table*}




\subsection{Video Examples}\label{v_examples}
We provide some video examples on DAVIS as follow. From the video comparison, it can be seen that the reconstructions of NeRV have lost spatial details, and it is difficult for DNeRV to reconstruct videos containing pervasive scattered high-frequency details. Whether there is large motion or high-frequency details in given videos, PNeRV is more robust in modeling the spatial consistency, leading to better perceptual quality in reconstructions. The links of examples are presented as follow.\\
Dance-jump: \url{https://drive.google.com/file/d/18JZq1BCkBJWCkZs-71OB7wI6j_Vma0vP/view?usp=drive_link}\\
Elephant: \url{https://drive.google.com/file/d/1rnPEsEtfA5UADU6BnwEDOPRG9hO9uPuM/view?usp=drive_link}\\
Kite-surf: \url{https://drive.google.com/file/d/1DDGw1zc2iJWcJHdBS4DOnfUQVf2H04Bs/view?usp=drive_link}\\
Parkour: \url{https://drive.google.com/file/d/1jWbJuoc-GCz2N_dXAJSER0PSy7ThrMr-/view?usp=drive_link}\\
Scooter-grey: \url{https://drive.google.com/file/d/1vs22Ru-AwAQuG710qbF72lwdHS1ABy83/view?usp=drive_link}




\section{Additional Ablation Studies}
\subsection{Visualization of Feature Maps}\label{app_fea}
To verify the effectiveness of hierarchical information merging by \textsc{KFc} and BSM, we visualize some feature maps in PNeRV-L which was pretrained on ``Parkour'' as examples. Those feature maps shown in Fig.~\ref{bsm_1} are in different channels and layers using the same frame as input. Those in Fig.~\ref{bsm_2} are all from the $4$-th layer but using different frames as input. The feature maps from $4$-th layer are in $480 \times 960$ and the original frames are in $960 \times 1920$. For each lower layer, the height and width are divided by 2 compared to the upper layer. ``Before'' and ``After'' means those feature maps are before passing through BSM or after.

Fig.~\ref{bsm_1} illustrates how the coarse features are refined by BSM. Different channels respond to distinct spatial patterns of video frames, including factors like color, geometric structure, texture, brightness, motion, and so forth. Before being processed by the BSM, the vanilla features are semantically mixed and entangled. However, the BSM is able to decouple these features and distinguish their specific effects, leading to more refined and distinct outputs.

Additionally, for imperfect feature maps, the BSM can add details or balance the focus of the reconstruction across various areas in the frames. These phenomena are commonly observed in the $4$-th layer, which is responsible for preparing for fine-grained reconstruction, as demonstrated in Figure.~\ref{bsm_2}. This shows the effectiveness of BSM in enhancing the quality of feature maps and in turn improving the overall reconstruction.


\subsection{Details of Model Structure}\label{app_det}
We ablate the structure details of PNeRV in 3M on ``Rollerblade'' in $480 \times 960$ from DAVIS, given in Tab.~\ref{abla_1}, Tab.~\ref{abla_2} and Tab.~\ref{abla_3}.
The alternation of kernel size or activation has little influence. Encoding more information into embeddings will help decoder reconstruct better, but also increase the overall size.

\subsection{Detailed Ablation Results of Proposed Modules on DAVIS}\label{app_dav}
To varify the contribution of different modules in PNeRV, we conduct ablation studies on (1) upscaling operators and (2) gated memory mechanisms. We compare KFc with two upscaling layers, Deconv and Bilinear, where ``Deconv'' is implemented by ``nn.ConvTranspose2d'' from PyTorch, and ``Bilinear'' is the combination of bilinear upsampling and Conv2D. KFc achieves better performance due to the global receptive field regardless of what fusion module it is combined with. 

Also, to illustrate the importance of adaptive feature fusion and improvement of BSM, we compare BSM with Concat, GRU and LSTM, where ``Concat'' means directly concatenate two features from different domain together. The ablation results suggest that, adaptive fusion of features from different domains significantly improves performance, and BSM outperforms other memory cells owing to the disentangled feature learning. The last row is the final PNeRV and the last column shows PSNR gaps when changing modules in PNeRV.


\begin{figure*}[t]
  \centering
  \includegraphics[width=0.95\linewidth]{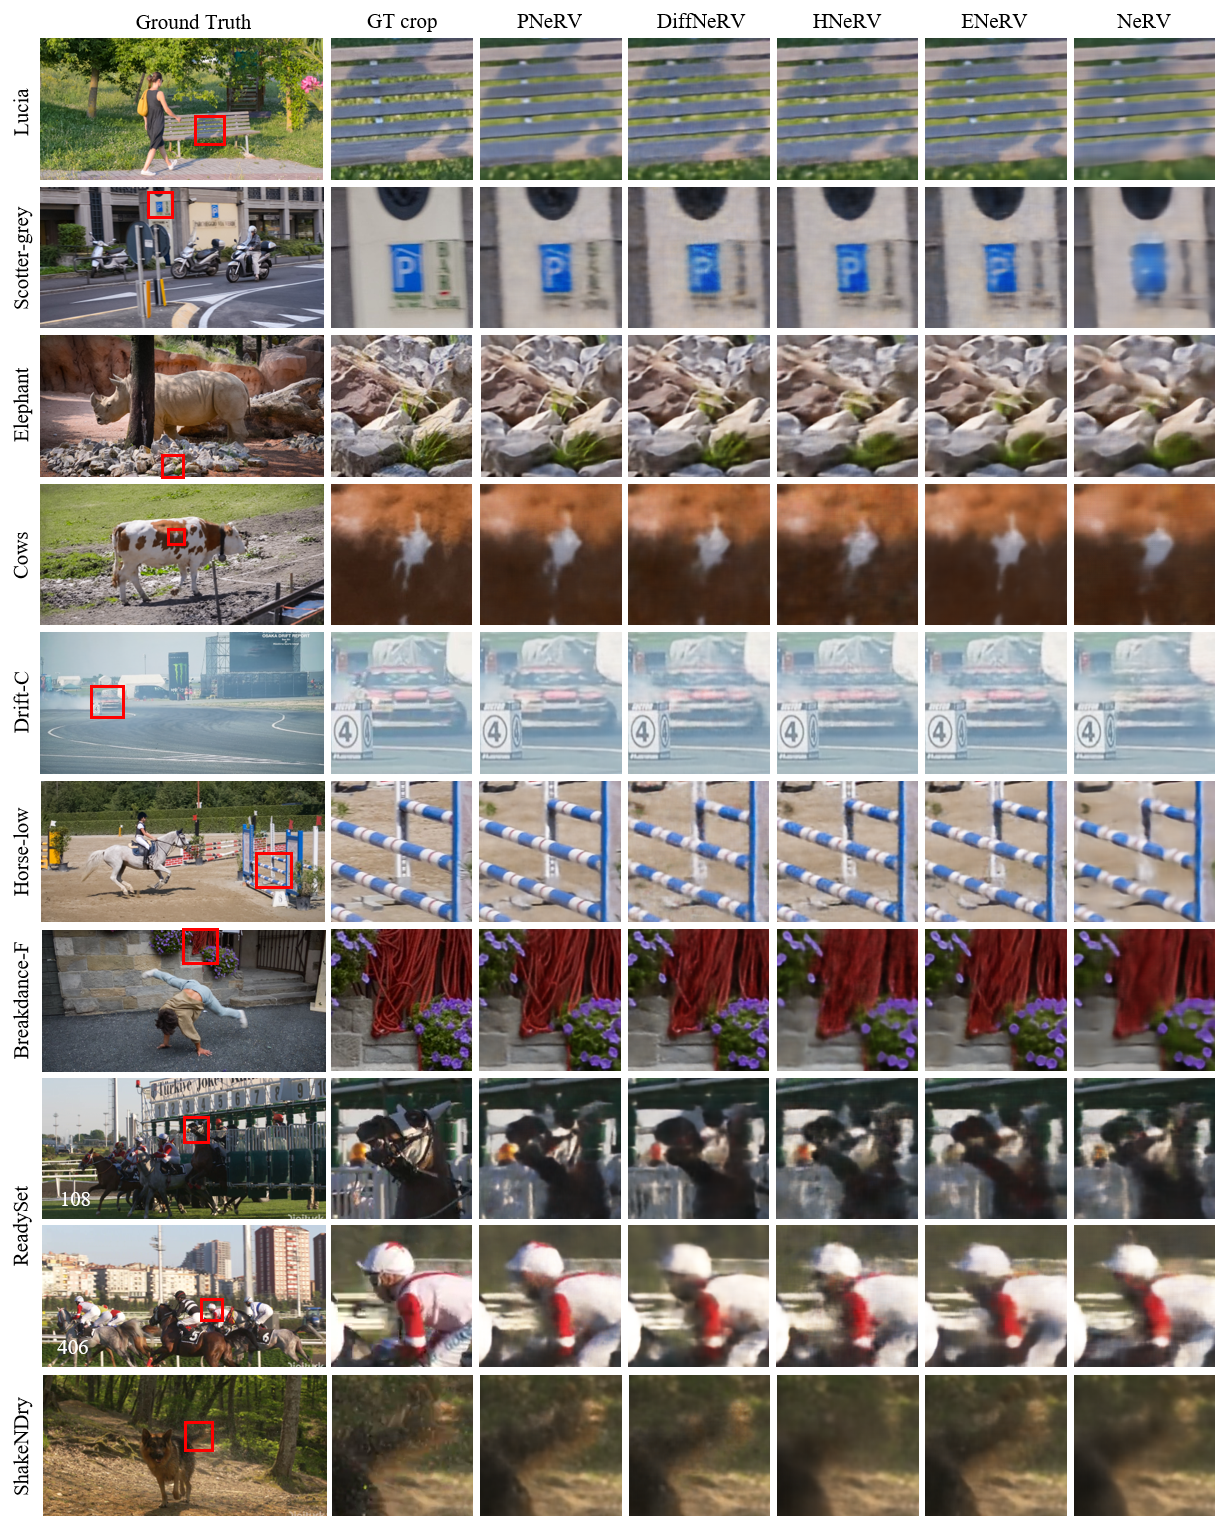}\\
  \vspace{-0.05in}\caption{Visual comparison examples on various videos.}
  \label{add_davis}%\vspace{-0.05in}
\end{figure*}


\begin{figure*}[t]
  \centering
  \includegraphics[width=0.95\linewidth]{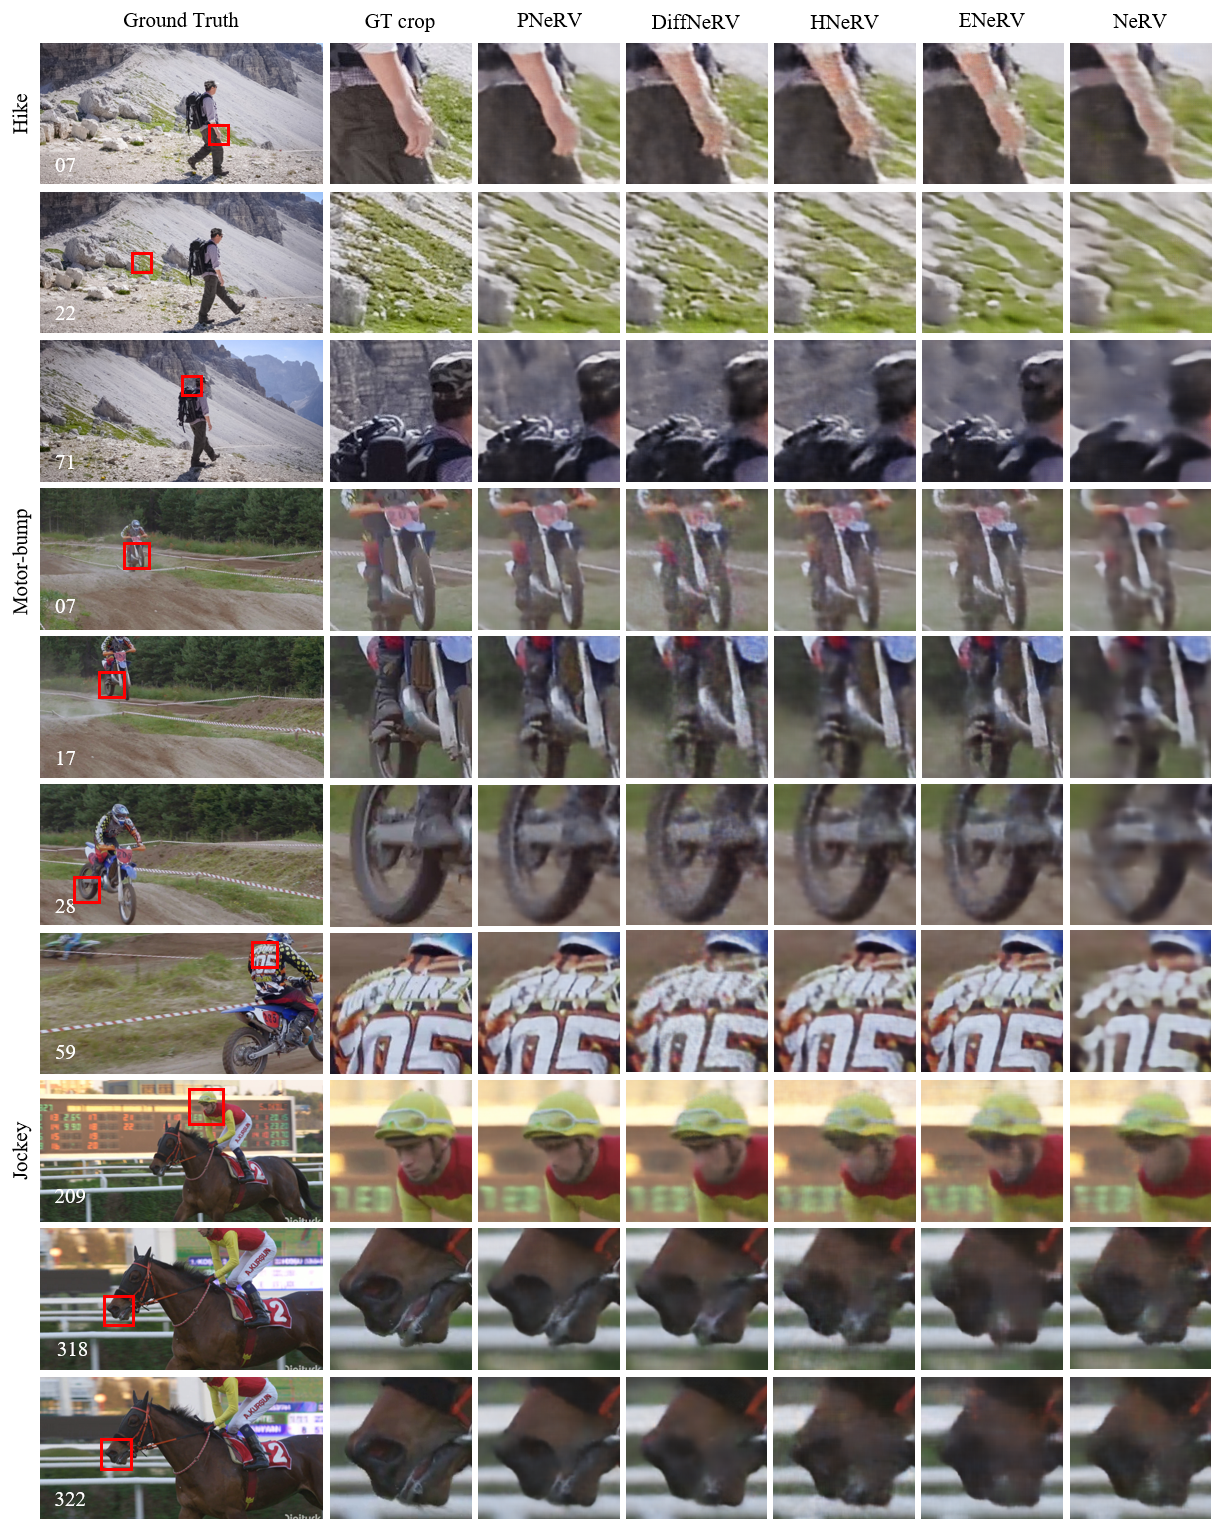}\\
  \vspace{-0.05in}\caption{Visual comparison examples on the same video by same models. Corresponding time stamps are shown in the bottom left.}
  \label{same_davis}%\vspace{-0.05in}
\end{figure*}


\begin{figure*}[t]
  \centering
  \includegraphics[width=1\linewidth]{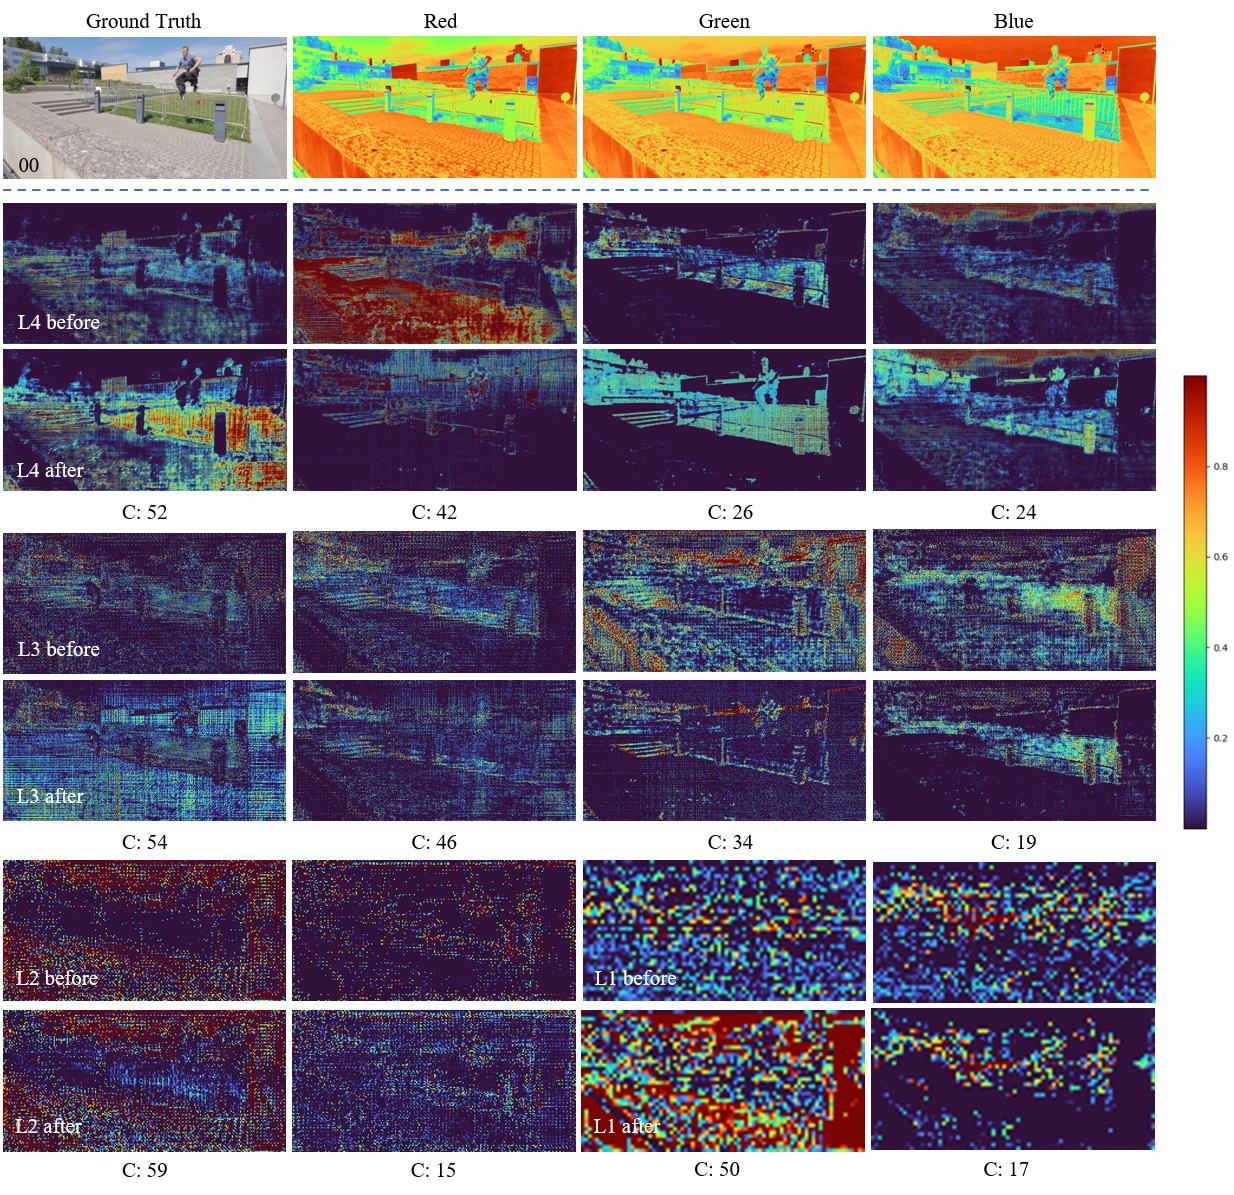}\\
  \vspace{-0.05in}\caption{Visualization examples of feature maps in different layers.``C'' refers to the channel number and ``L'' is the layer number.}
  \label{bsm_1}%\vspace{-0.05in}
\end{figure*}

\begin{figure*}[t]
  \centering
  \includegraphics[width=1\linewidth]{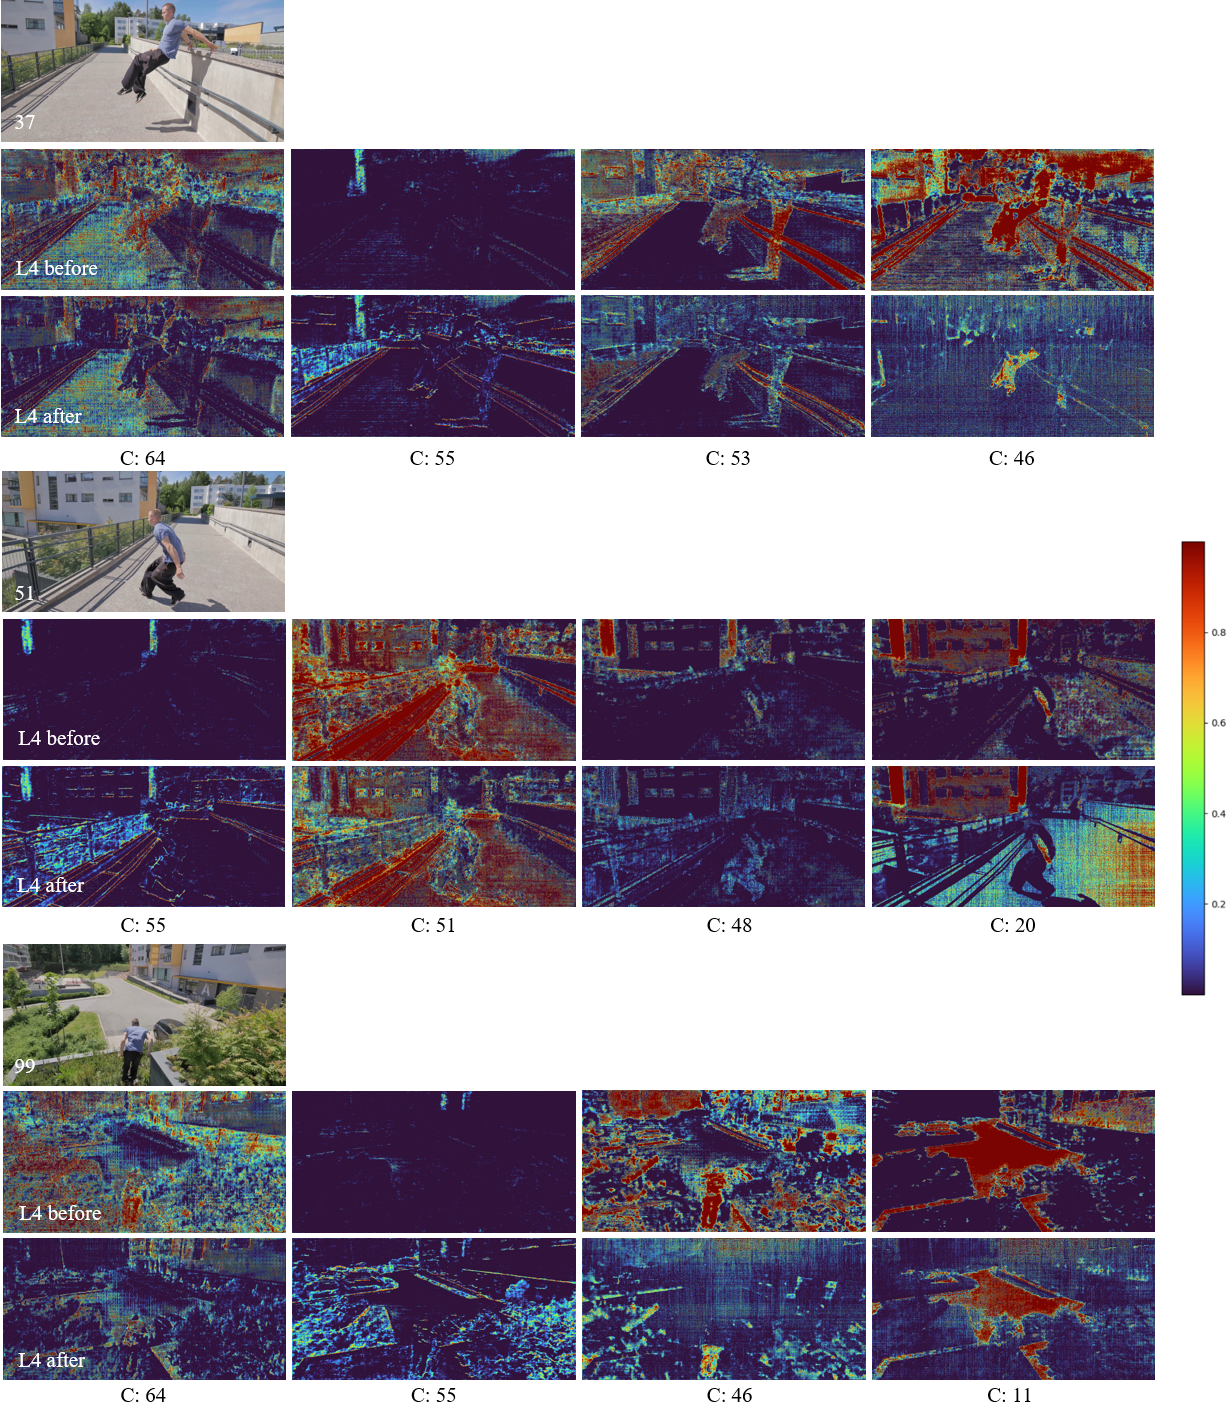}\\
  \vspace{-0.05in}\caption{Visualization examples of feature maps for different frames.``C'' refers to the channel number and ``L'' is the layer number.}
  \label{bsm_2}%\vspace{-0.05in}
\end{figure*}



\iffalse
\section{Pseudocode}
The proposed PNeRV framework is easy to be implemented based on the commonly-used layers. We provide a PyTorch-like pseudocode of
\textsc{KFc} and single layer in PNeRV as follow.

\begin{python}\scriptsize
import torch
import torch.nn as nn
class KFc(nn.Module):
	def __init__(self, in_height, in_width, out_height, out_width, channels):
		super().__init__()
		self.in_h = in_height
		self.in_w = in_width
		self.out_h = out_height
		self.out_w = out_width
		self.c = channels

		self.w_L_ = torch.zeros(self.c, self.out_h, self.in_h)
		self.w_R_ = torch.zeros(self.c, self.in_w, self.out_w)
		nn.init.kaiming_normal_(self.w_L_, mode='fan_out', nonlinearity='relu')
		nn.init.kaiming_normal_(self.w_R_, mode='fan_out', nonlinearity='relu')
		self.w_L = nn.Parameter(self.w_L_)
		self.w_R = nn.Parameter(self.w_R_)

		self.b_h = nn.Parameter(torch.zeros(self.out_h, 1))
		self.b_w = nn.Parameter(torch.zeros(1, self.out_w))
		self.b_c = nn.Parameter(torch.zeros(self.c, 1))

	def forward(self, x):
		b_ = self.b_h @ self.b_w
		b__ = b_.reshape(1, self.out_h*self.out_w)
		_ = self.b_c @ b__
		__ = _.reshape(self.c, self.out_h, self.out_w)
		b = __.repeat(self.in_b, 1, 1, 1)
		_ = torch.matmul(self.w_L, x)
		return torch.matmul(_, self.w_R) + b

def PNeRV_one_layer(embedding, input):
    c,h,w = embedding.shape
    C,H,W = input.shape

    #KFc layer
    pym = KFc(h, w, H, W, c)(embedding)
    pym = nn.BatchNorm2d(c, track_running_stats=True)(pym)
    pym = nn.GELU()(pym)

    #BSM layer
    memory = nn.Conv2d(C, C, 3, 1, 1)(input)
    kownledge = nn.Conv2d(c, C, 3, 1, 1)(pym)
    _ = torch.relu(memory + kownledge)
    decision = torch.sigmoid(nn.Conv2d(C, C, 3, 1, 1)(_))
    output = decision * knowledge + (1- decision) * input

    #We did not do extra modification on basic NeRV block.
    ruturn NeRV_block(output)
\end{python}
\fi

\iffalse
\clearpage
\setcounter{table}{0}
\renewcommand\thetable{A.\arabic{table}}


\section{Response Overview}

\textbf{Summary}. We thank the reviewers for their constructive comments. We are glad that reviewers agree with introducing Universal Approximation Theory (UAT) into video Implicit Neural Representation (INR)(``a good attempt for this research area'' (kUsn), ``a unique and novel contribution''(Uyr4)). We're further glad that reviewers agree that PNeRV shows improvements compared to state-of-the-art (sota) methods (``sound reasonble''(kUsn), ``showing potential to compete with previously methods''(BhmE) and ``results are extensive'' (4rj7)). Regarding some common concerns and misunderstandings which reviewers raise, we would like to offer several clarifications first. We use the reference number from the main paper in the Response.

\subsection{Discussion of the motivation of pyramidal design and the connection from theoretical analysis to it (kUsn, BhmE, 4rj7).}
In fact, the pyramidal design is clearly guided by theoretical analysis. According to Theorem 1, the upper bound of the minimal parameters under certain approximation error is **fixed** once the decoder blocks are cascaded regardless of the module's details (channels or kernel size), resulting in limited approximation ability. But according to Theorem 3.1 in ''Resnet with one-neuron hidden layers is a universal approximator'' [14] or Theorem 1 in ''Universal approximation by a slim network with sparse shortcut connections'' [15] (as we claimed in Line 182), the model with residual connection will reduce the maximum width of layers to 1 under the same condition. Differing from the minimal width given in Lemma 1, the model with only one-neuron hidden layers could achieve universal ability. This means that the model size can be greatly reduced but maintain the performance by shortcut connection.

Towards the significance of shortcut connection, next question is how to use it reasonably to enhance the approximation ability. Meanwhile, we found that existing videoINRs could hardly model the complicated spatiotemporal continuity well (visualizations in Fig. 3 of main paper and Fig. 2 of appendix). To address these, pyramidal structure is the key. In PNeRV, the low-dim features with high-level global information will guide the higher-dim fine-grained features in shortcut connections. With the help of the pyramidal design, the model not only improves its approximation ability, but also obtains a global receptive field, which can address the dilemma of spatial discontinuity in existing NeRV systems.

\subsection{Discussion of the motivation of KFc and its efficiency (kUsn, Uyr4).}
As we discussed above, the key to the videoINRs' improvement is adding shortcut connection in decoder to form a pyramidal structure instead of using only cascaded layers which adopted in NeRV [7] or HNeRV [17]. This is a non-trivial challenging but underappreciated matter, owing to two critical constraints: (1) model size limit and (2) enormous scaling ratio. Using as few parameters as possible to represent videos is the pursuit of videoINR, better performance under the same model size indicates that the model is more efficient (namely Dual INVC problem in Lines 134-136). Also, NeRV systems aim to encode high-resolution realistic videos ($960\times1920$) efficiently through extremely small embedding per frame, once upscaling tiny bottom embedding to upper layers, the scaling ratio will be dramatically big.

Under these constraints, the upscaling operators based on subpixel filling are failed, which was discussed in Line 198-207. Once upscaling from tiny embeddings $F_0$ ($16\times2\times4$) to fine-grained features $F_n (16\times 320\times 640)$, it needs unbearable huge numbers of channels to fill in target subpixels. For example, when kernel size is only $1\times1$, a single PixelShuffle layer requires 6.96M parameters from $F_0$ to $F_n$. An efficient upscaling operator under this situation is urgently needed.

KFc is motivated by that, **the subpixels of one position in larger resolution are related to every position in current feature map, differ from surrounding positions in Deconv or PixelShuffle**. Through $K_1 \cdot F_0 \cdot K_2$, where $\cdot$ denotes matrix multiplication, $K_1 $ in $16\times320\times2$ and $K_2 $ in $16\times4\times640$, an efficient rescaling is achieved (further we add a bias term). The parameters of KFc from $F_0$ to $F_n$ is only 0.05M, only $\textbf{0.7\%}$ of PixelShuffle under same condition. As a lightweight upscaling operator, KFc could realize the efficient rescaling when scaling ratio is huge, becomes the fundamental modules of pyramidal design.

\subsection{Discussion of the main challenge in videoINR and the performance comparison (kUsn, 4rj7).}
We would like to reemphasize the challenge of videoINR. Different from INR on 3D generation or rendering, videoINR attempts to achieve better reconstruction with a fixed amount of parameters, while it is quite difficult according to Rate-Distortion theory. At a fixed bit rate, there exists an upper limit to the PSNR. In addition, according to Rate-Distortion-Perception theory (``Rethinking lossy compression: The rate-distortion-perception tradeoff, ICML2019''), there exists a tradeoff between distortion and perception. The pyramidal architecture is beneficial to improve perception performance owing to global receptive field, and the LPIPS results given in Tab. 2 of appendix, visualizations shown in Fig. 3 of main paper and Fig. 2 of appendix all prove the improvement of PNeRV in perception. Although PSNR increase seems not to big, but the perception performance achieves a great improvement. PSNR is not the only metric to compare performance (although PNeRV-M shows $\textbf{+1.96}$ improvement against baseline HNeRV), and PNeRV achieves best results on PSNR, LPIPS and FVD ($\textbf{+23.2\%}$), shown in Tab.A.2. In conclusion, a small step of PSNR increase, a huge step for videoINR.

Additional results are given in attachment where ablations on Tab. A.1 and FVD on Tab.A.2. Thank again for all your constructive and helpful comments.
\fi



%29.78/0.885
%30.99/0.898




\iffalse
\begin{figure}[t]
    \centering
	\begin{minipage}{1\linewidth}
		\centering
		\vspace{-0.07in}
		\setlength{\abovecaptionskip}{0.5cm}
		\includegraphics[width=\linewidth]{comp.png}
 	   \vspace{-0.24in}
		\caption{Comparison of video compression on UVG.}

		\label{comp}
	\end{minipage}
\vspace{-0.05in}
	%\qquad
	\hfill

\end{figure}


\begin{table}[h]\small
    \tabcolsep=0.1cm
      \setlength{\abovecaptionskip}{5pt}
      \caption{FVD comparison on UVG, the smaller the better. We only compare PNeRV with DiffNeRV because it outperforms other NeRV methods. PNeRV achieves better results on most of the videos. Although DiffNeRV has better PSNR results on ``Beauty'' and ``YachtR'', PNeRV's reconstructions gain significant improvement (\textbf{+23.2\%}) in perception quality and spatiotemporal coherence modeling. PNeRV outperforms the sota NeRV methods on PSNR, LPIPS and FVD.}
      %\resizebox{!}{1.05cm}{
      \centering
  \begin{tabular}{l||lllllll|c}
 %\toprule
     \textit{FVD}    $\downarrow$      & Beauty & Bospho & HoneyB & Jockey & ReadyS & ShakeN &YachtR &Avg.\\
    \midrule[0.8pt]
    DiffNeRV~\cite{DNeRV}&1.29e-5 &4.28e-5 &6.50e-6 &1.55e-4 &6.58e-4 &4.69e-5 &2.23e-4 &-\\
    PNeRV              &9.88e-6 &2.85e-5 &4.96e-6 &9.70e-5 &8.94e-4 &1.17e-5 &2.11e-4 &-\\
    \midrule[0.1pt]
    Improvement          &+23.4\%  &+33.4\%  &+23.7\% &+37.4\% &-35.8\% &+75.0\% & +5.4\% & \textbf{+23.2\%}\\
       \midrule[0.8pt]
         \textit{LPIPS} $\downarrow$ &&&&&&&& \\
              \midrule[0.1pt]
    DiffNeRV~\cite{DNeRV}  &0.205 &0.164 &0.042 &0.164 &0.206 &0.181 &0.241 &0.172\\
    PNeRV                &0.210	&0.132 &0.037 &0.177 &0.211 &0.146 &0.230 &\textbf{0.163}\\

   \midrule[0.8pt]
   \textit{ PSNR }$\uparrow$ &&&&&&&& \\
              \midrule[0.1pt]
    DiffNeRV~\cite{DNeRV}  &40.00 &36.67 &41.92 &35.75 &28.67 &36.53 &31.10 &35.80\\
    PNeRV                &38.94	&36.68 &42.73 &35.81 &28.97 &38.25 &30.92 &\textbf{36.04}\\

   \bottomrule[0.8pt]
  \end{tabular}%}
  \label{LPIPS}
\end{table}
\fi
